# Supplementary material for: Accelerating COVID-19 research with graph mining and transformer-based learning
Source: arXiv:2102.07631 source file (2021-09-29)
Supplement: Supplementary file 1 [file appendix.tex]

\section{Augmenting Semantic Predicates: Deployment Details}

The RnnOIE model by Stanovsky \emph{et al.} uses a deep Bi-LSTM~\cite{Schuster} model to learn the joint word embedding and predict the resulting semantic position tags. Since LSTMs are inherently sequential model, it means that the inference time per sentence would be considerable. We first tried processing an entire collection of abstracts at once on a cluster of 10 machines each consisting of 24 CPUs using the \texttt{Dask}~\cite{matthew_rocklin-proc-scipy-2015} library. The entire process took more than 8 hours. Considering that we had about 100 such collections, this inference time was prohibitively high. In order to speed up inference we read each collection once and distributed chunks of abstracts over the machines. This change helped us to cut down the processing time from over a week to just over 4 days for the MEDLINE corpus. For the CORD-19 corpus the processing time was even faster at 2 days.  The next step was to align the extracted predicates with the \texttt{SemRep} recognized biomedical concepts. We achieved this alignment by first building an index of files that contained a specific abstract ID and then processing the RnnOIE predicates with the aforementioned index. We further optimized the indexing phase by updating the existing index each time we processed more than $\tau$ abstracts.

The semnet filter does not introduce additional computational overhead and can process a thousand abstracts in under 1 second. Hence, to obtain the most relevant set of predicates we were able to parallelize over  ``checkpoints" (each of which contained ~30k abstracts) in an hour.
